# Supplementary material for: Aviary: training language agents on challenging scientific tasks
Source: arXiv:2412.21154 source file (2024-12-30)
Supplement: Supplementary file 1 [file appendix.tex]

\section{Poisson Gradient Estimation}
\label{appendix:gradient_estimation_poisson}

Analytical derivation of the gradient of the graph in \autoref{subsection:gradient_estimation_poisson}.

\begin{align*}
    & \nabla_k \mathbb{E}_{x \sim \text{Poisson}(k)} [L] = \nabla_k \sum P(x \mid k) \cdot L \, && \text{(by definition of expectation)} \\
    &= \sum \left( \nabla_k P(x \mid k) \cdot L + P(x \mid k) \cdot \nabla_k L \right) && \text{(product rule for differentiation)} \\
    &= \sum \left( P(x \mid k) \cdot \nabla_k L + L \cdot \nabla_k P(x \mid k) \right) && \text{(reordering terms for readability)} \\
    &= \sum P(x \mid k) \cdot \left( \nabla_k L + L \cdot \nabla_k \ln P(x \mid k) \right) && \text{(using } \nabla_k P(x \mid k) = P(x \mid k) \cdot \nabla_k \ln P(x \mid k)\text{)} \\
    &= \mathbb{E}_{x \sim \text{Poisson}(k)} \left[ \cancel{\nabla_k L} + L \cdot \nabla_k \ln P(x \mid k) \right] && \text{(since } L \text{ does not directly depend on } k\text{)} \\
    &= \mathbb{E}_{x \sim \text{Poisson}(k)} \left[ L \cdot \nabla_k \ln P(x \mid k) \right]
\end{align*}

The loss function used is our experiment is $L(x) = |x - t|$ where $t$ is the target value. We use an SGD optimizer, a learning rate of 0.01, and a batch size of 8.

\begin{figure}[htbp]
    \centering
    \includegraphics[width=\linewidth]{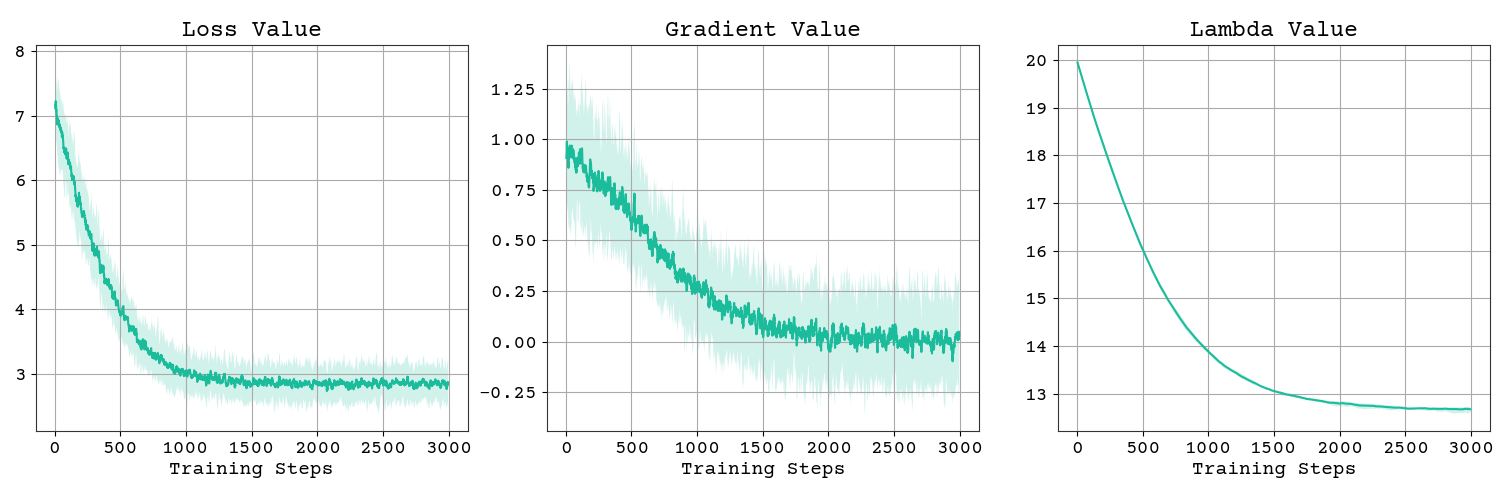}
    \caption{Poisson example optimization curves. The target value $t$ is 13 and the initial $k$ value is 20. We ran the experiment 5 times and report the mean, with shaded areas representing the maximum and minimum values observed.}
    \label{fig:poisson_optimization}
\end{figure}

\pagebreak

\section{Black Box Gradient Estimation}
\label{appendix:gradient_estimation_llm}

The analytical derivation of the API call's configuration (Cfg) gradient for the Black Box example in ~\autoref{subsection:gradient_estimation_llm} is analogous to that of the Poisson graph, but we cannot compute it because API calls to language models typically return only the output value. However, if we obtain a good enough approximation, our framework allows it to be used in the backward pass.

\vspace{0.1cm}
\[
\nabla_{\text{Cfg}} \mathbb{E}[L] = \mathbb{E}\left[L \nabla_{\text{Cfg}} \ln P(x \mid \text{Cfg})\right] 
\]
\vspace{0.1cm}

To approximate the gradients, we train a Multi-Layer Perceptron (MLP) to model the behavior of the LLM given the Cfg using supervised learning. Noise (±2 token limit) is added to the configuration, and we predict the embedded LLM output. Mean Squared Error (MSE) loss is used to train the MLP. The diagram below illustrates this process.

\vspace{0.5cm}
\begin{tikzpicture}[scale=0.5, node distance=1.5cm and 1.5cm]
    \tikzstyle{det} = [rectangle, draw, text centered, inner sep=3]
    \tikzstyle{stoch} = [rectangle, draw, dashed, text centered, inner sep=5]
    \tikzstyle{line} = [draw, -{Stealth[length=3mm, width=2mm]}]

    % Nodes
    \node[det] (config) at (0,0) {$\text{Cfg}$};
    \node[det, right=0.7cm of config] (noisy_config) {$\text{NoisyCfg} = \text{Cfg} + \text{Noise}$};

    % MLP node, diagonally up and right from noisy_config
    \node[det, right=0.7cm of noisy_config, yshift=1.5cm] (mlp) {$\hat{e}_\text{MLP} = \text{MLP(NoisyCfg)}$};

    % LLM node, diagonally down and right from noisy_config
    \node[stoch, right=-0.5cm of noisy_config, yshift=-1.5cm] (llm) {$\hat{a} \sim \text{LLM(NoisyCfg)}$};

    % Embedding node after LLM turning a into e
    \node[det, right=0.5cm of llm] (embedding) {$\hat{e}$ = Embedding($\hat{a}$)};

    % Loss node at the same level as config, diagonally to the right of MLP and LLM
    \node[det, right=0.2cm of embedding, yshift=1.5cm] (loss1) {$L = \text{Loss}(\hat{e}_\text{MLP}, \hat{e})$};

    % Paths
    \path[line] (config) -- (noisy_config);
    \path[line] (noisy_config) -- (mlp);
    \path[line] (noisy_config) -- (llm);
    \path[line] (llm) -- (embedding);

    \path[line] (mlp) -- (loss1);
    \path[line] (embedding) -- (loss1);
\end{tikzpicture}
\vspace{0.5cm}

For simplicity, we omit the following detail in the graph: the Cfg actually contains both the prompt and the parameter to be optimized, which is the token limit. We embed the prompt and concatenate it with the token limit value before passing it to the MLP. When computing the gradient, we only compute it with respect to the token limit parameter.

To account for changes in LLM behavior after updating configuration values, we alternate between 10 training updates for the MLP and 10 updates to the configuration values. Initially, we perform 300 MLP training steps. We introduce noise of ±2 tokens to explore the effects of different token limits while we do not change the prompt. The language model used is OpenAI's \texttt{gpt-4o-mini-2024-07-18}. The text embeddings have a size of 512, and they are obtained using OpenAI's \texttt{text-embedding-3-small} model. The MLP has 2 hidden layers, each with a size of 512, followed by layer normalization~\cite{lei2016layer} and a final layer that predicts the mean and standard deviation of the output. We use the reparameterization trick to sample the output. An Adam optimizer~\cite{kingma2014adam} is used to train the MLP with a learning rate of 0.0005, while a simple SGD optimizer is used to train the token limit parameter with a learning rate of 10.

\begin{figure}[h!]
    \centering
    \includegraphics[width=\linewidth]{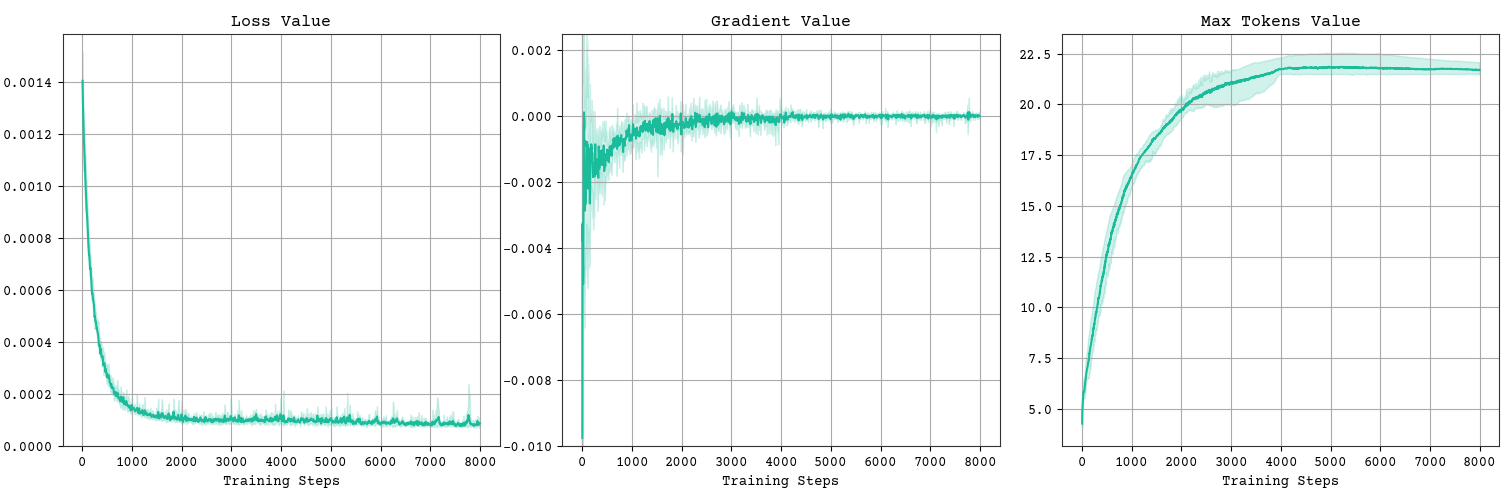}
    \caption{Black box optimization curves. The loss decreases rapidly and converges near zero. The gradient decreases to zero as the learning process stabilizes. The max token value increases from the initial value of 4 to over 20, then stabilizes as gradients diminish. Shaded areas indicate minimum and maximum values across 5 random seeds.}
    \label{fig:black_box_optimization}
\end{figure}
